# Supplementary material for: Unsupervised Network Embedding Beyond Homophily
Source: arXiv:2203.10866 source file (2022-12-22)
Supplement: Supplementary file 2 [file appendix_synthetic_data_generation.tex]

\section{Synthetic Dataset Generation}
\label{sec:appendix_syn_data_generation}
We generate $10$ random synthetic networks (synthetic-$h$) with various homophily levels $h$ and node features by adopting a similar approach to~\cite{APKALHSG19,KO21}.
Specifically, each synthetic network has $10$ classes and $500$ nodes per class. 
Nodes are assigned random features sampled from 2D Gaussians.

\smallskip\noindent
\textit{Network generation}.
We generate synthetic network $\mathcal{G}$ of $|\mathcal{V}|$ nodes with $|\mathcal{Y}|$ different class labels, and $\mathcal{G}$ has $|\mathcal{V}|/|\mathcal{Y}|$ nodes per class. 
$|\mathcal{V}|$ and $|\mathcal{Y}|$ are two prescribed numbers to determine the size of $\mathcal{G}$. 
Synthetic network's homophily ratio $h$ is mainly controlled by $p_{in}$ and $p_{out}$, where $p_{in}$ means the possibility of existing an edge between two nodes with the same label and $p_{out}$ is the possibility of existing an edge between two nodes with different labels. 
Furthermore, the average degree of $\mathcal{G}$ is $d_{avg}=|\mathcal{V}|/|\mathcal{Y}| \cdot \delta$, where $\delta = p_{in} + (|\mathcal{Y}|-1) \cdot p_{out}$. 
Following the described network generation process, with given $|\mathcal{V}|$, $\mathcal{Y}$ and $d_{avg}$, we choose $p_{in}$ from $\{0.0001\delta, 0.1\delta, 0.2\delta, \dots, 0.9\delta \}$. 
Note that the synthetic network generation process requires both $p_{in}$ and $p_{out}$ are positive numbers, hence we use $p_{in}=0.0001\delta$ to estimate $h=0$ case.
